# Supplementary material for: One Teacher is Enough? Pre-trained Language Model Distillation from Multiple Teachers
Source: arXiv:2106.01023 source file (2021-06-02)
Supplement: Supplementary file 1 [file supplement.tex]

\section*{Supplementary Materials}

\subsection*{Experimental Environment}

Our experiments are conducted on a cloud Linux (Ubuntu 16.04) server.
The version of Python is 3.6 and we implement our experiments with Pytorch 1.2.0.
The server has 4 Tesla V100 GPUs, each of them has 32 GB memory.
We use the horovod library to conduct experiments on multiple GPUs in parallel.

\subsection*{Preprocessing}
The effort on preprocessing in our approach is minimal.
We use the transformers package to implement our experiments.
We use the word piece tokenizer in this package for word tokenization, and we limit the maximum number of tokens to 64.
We do not filter low frequency tokens in our approach.
The token sequences are padded to the same length with the zero padding tokens.

\subsection*{Hyperparameter Settings}

The detailed hyperparameter settings are listed in Table~\ref{hyper}.

\begin{table}[h]
\centering
%\resizebox{1.0\linewidth}{!}{
\begin{tabular}{|l|c|}
\hline
\multicolumn{1}{|c|}{\textbf{Hyperparameters}}& \textbf{Value} \\ \hline
hidden dimension                     & 768            \\ 
attention query dimension                     & 200            \\ 
dropout                                      & 0.2            \\
optimizer                                    & Adam           \\
teacher model learning rate                                & 2e-6           \\
student model learning rate                                & 5e-6           \\
batch size                                   & 64    \\   
\hline
\end{tabular}
%}
\caption{Detailed hyperparameter settings.}\label{hyper}
\end{table}

\subsection*{Model Initialization}

We use the embedding and first 4 or 6 Transformer layers of UniLM to initialize the parameters in the student model rather than train it from scratch.
We find using the  first $K$ layers of the teacher model for initialization is better than using the last $K$ layers or the skip scheme used in BERT-PKD. 

\subsection*{Notes on Pooling}

In our experiments, we find the model performance of using the hidden representation of the ``[CLS]'' token is not satisfactory.
Thus, we choose to pool the entire hidden representation sequence output by the model.
We find that attentive pooling achieves better performance than average or max pooling.
